# Supplementary material for: Feedback Control For Cassie With Deep Reinforcement Learning
Source: arXiv:1803.05580 source file (2018-07-27)
Supplement: Supplementary file 1 [file appendix.tex]

\section{Reward Function Design}
